# Supplementary material for: GREENER: A Tool for Improving Energy Efficiency of Register Files
Source: arXiv:1709.04697 source file (2018-03-29)
Supplement: Supplementary file 1 [file 11-Appendix.tex]

\appendix
\begin{figure*}
\centering
\includegraphics[scale=0.45]{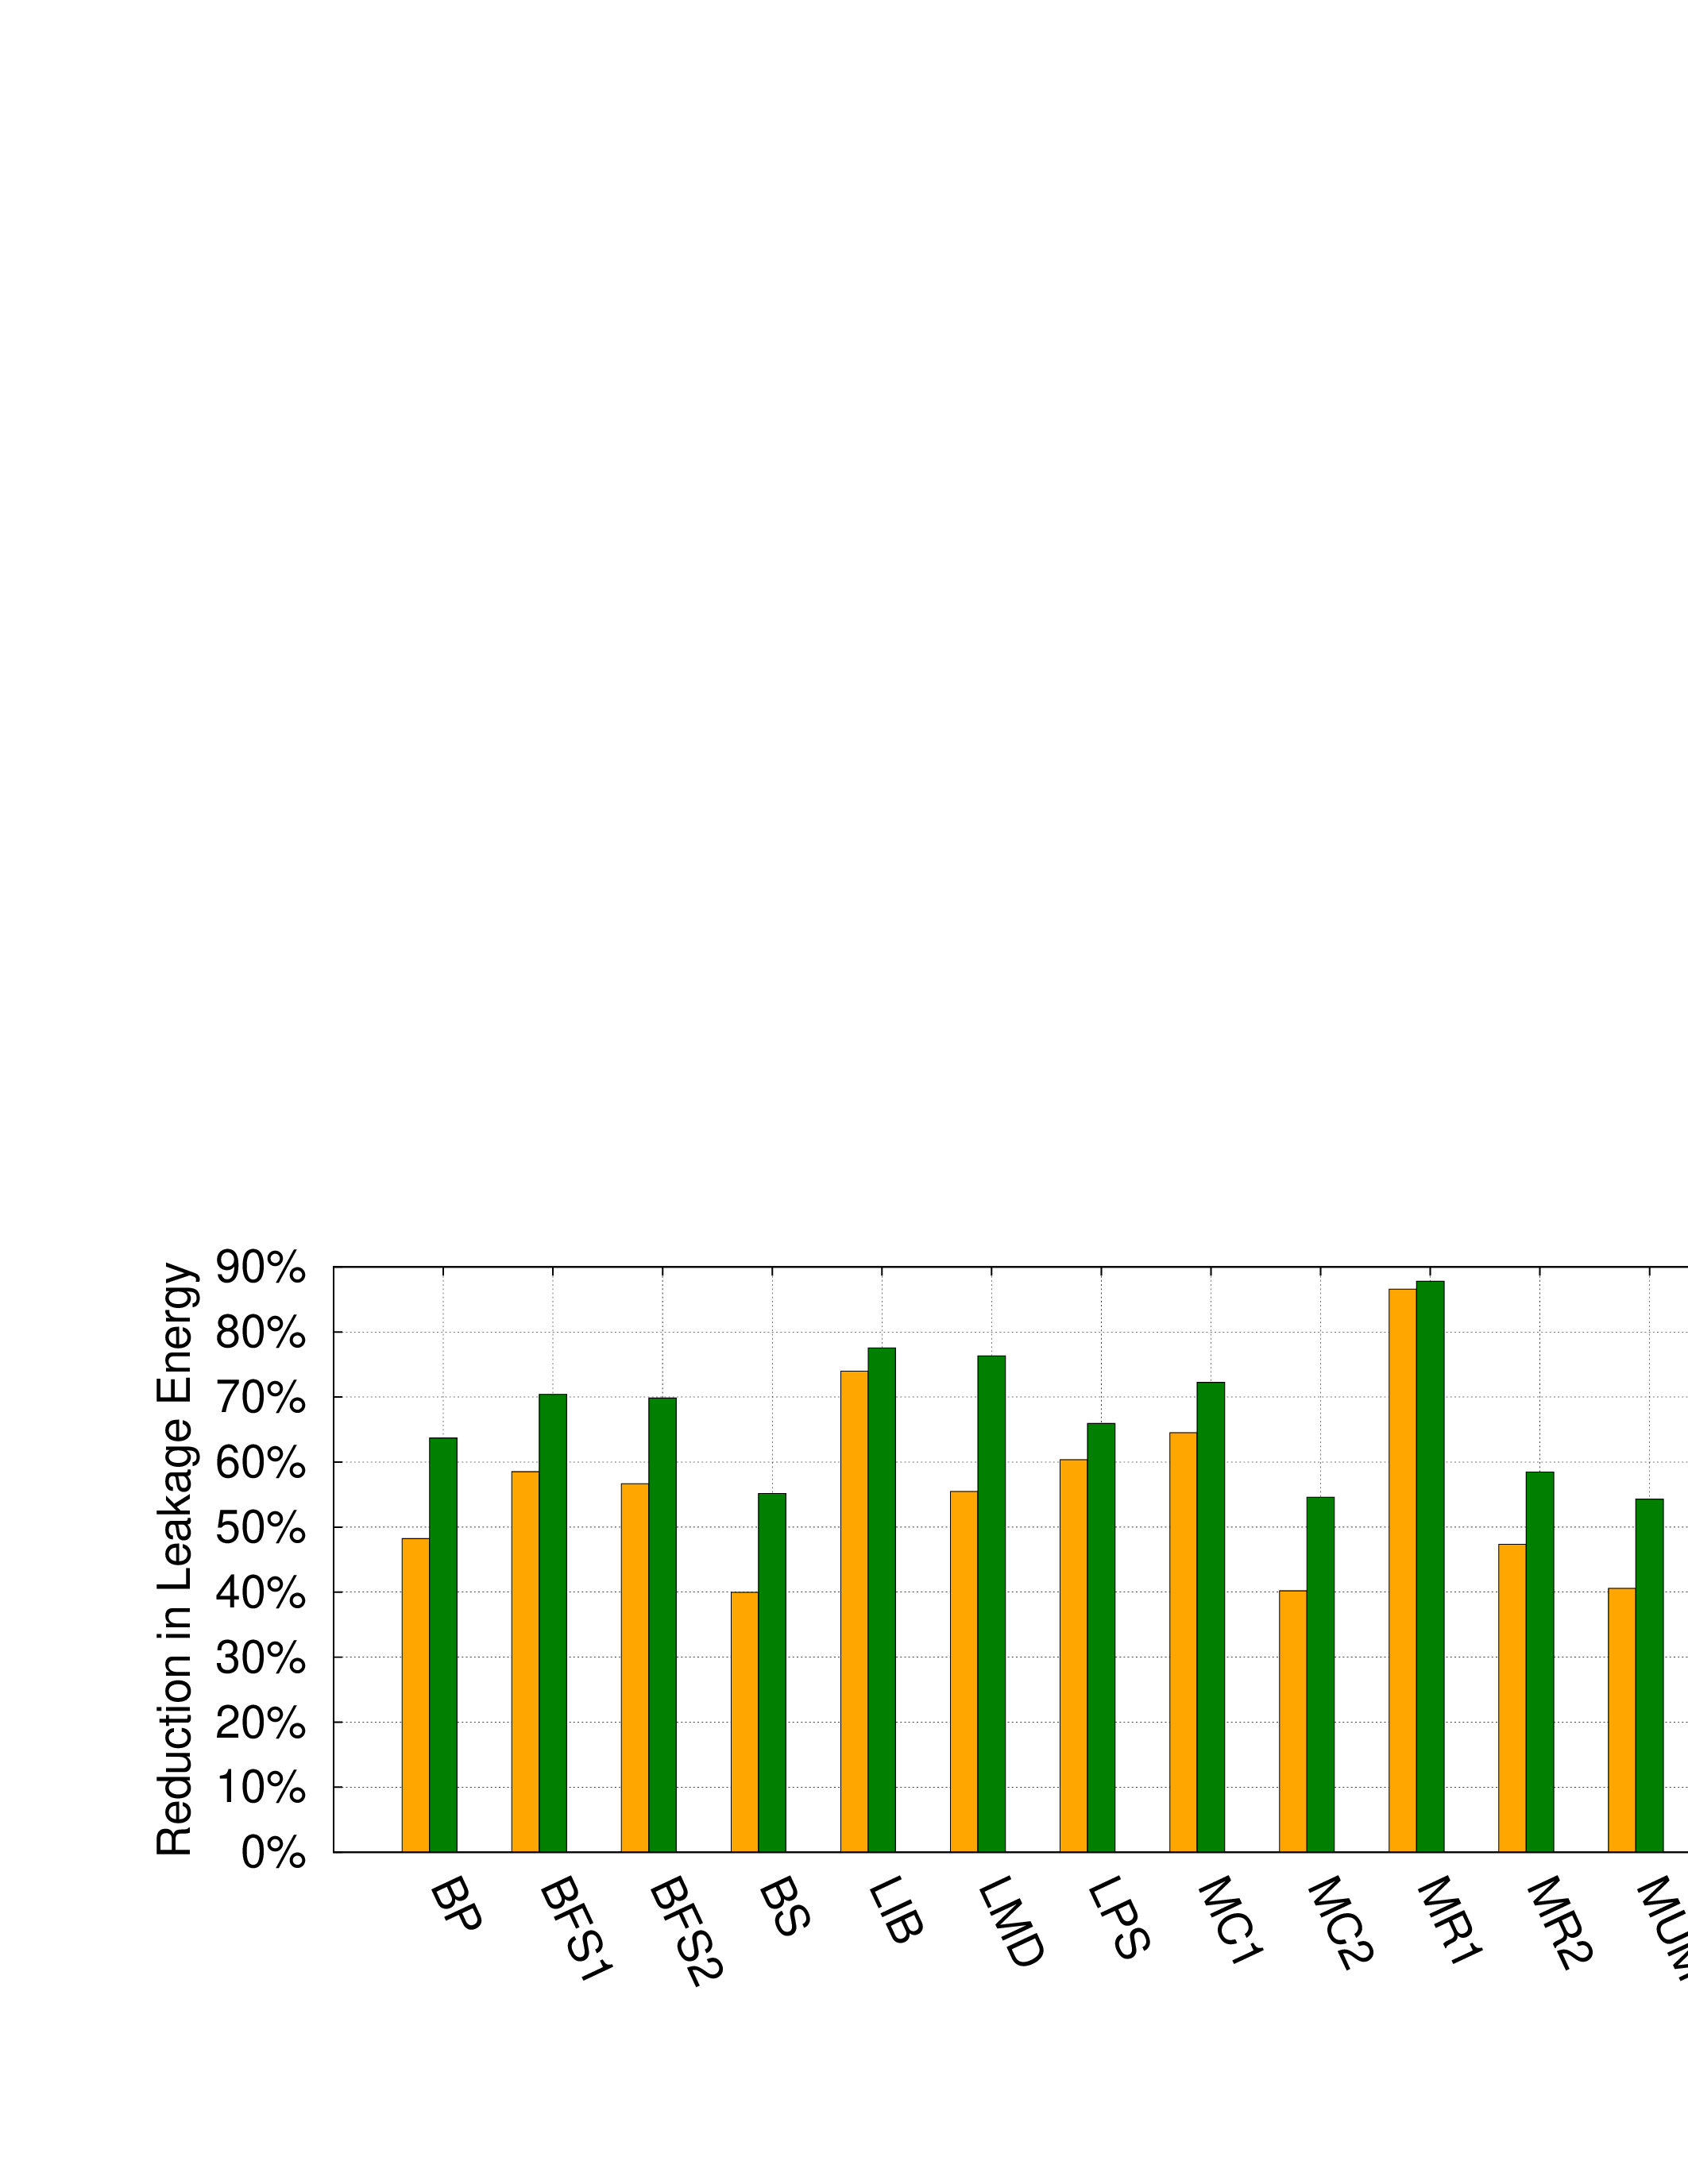}
\vskip -3mm
\caption{Comparing Leakage Energy with GTO Scheduler}
\label{fig:GTO}
\vskip -3mm
\end{figure*}

\begin{figure*}
\centering
\includegraphics[scale=0.45]{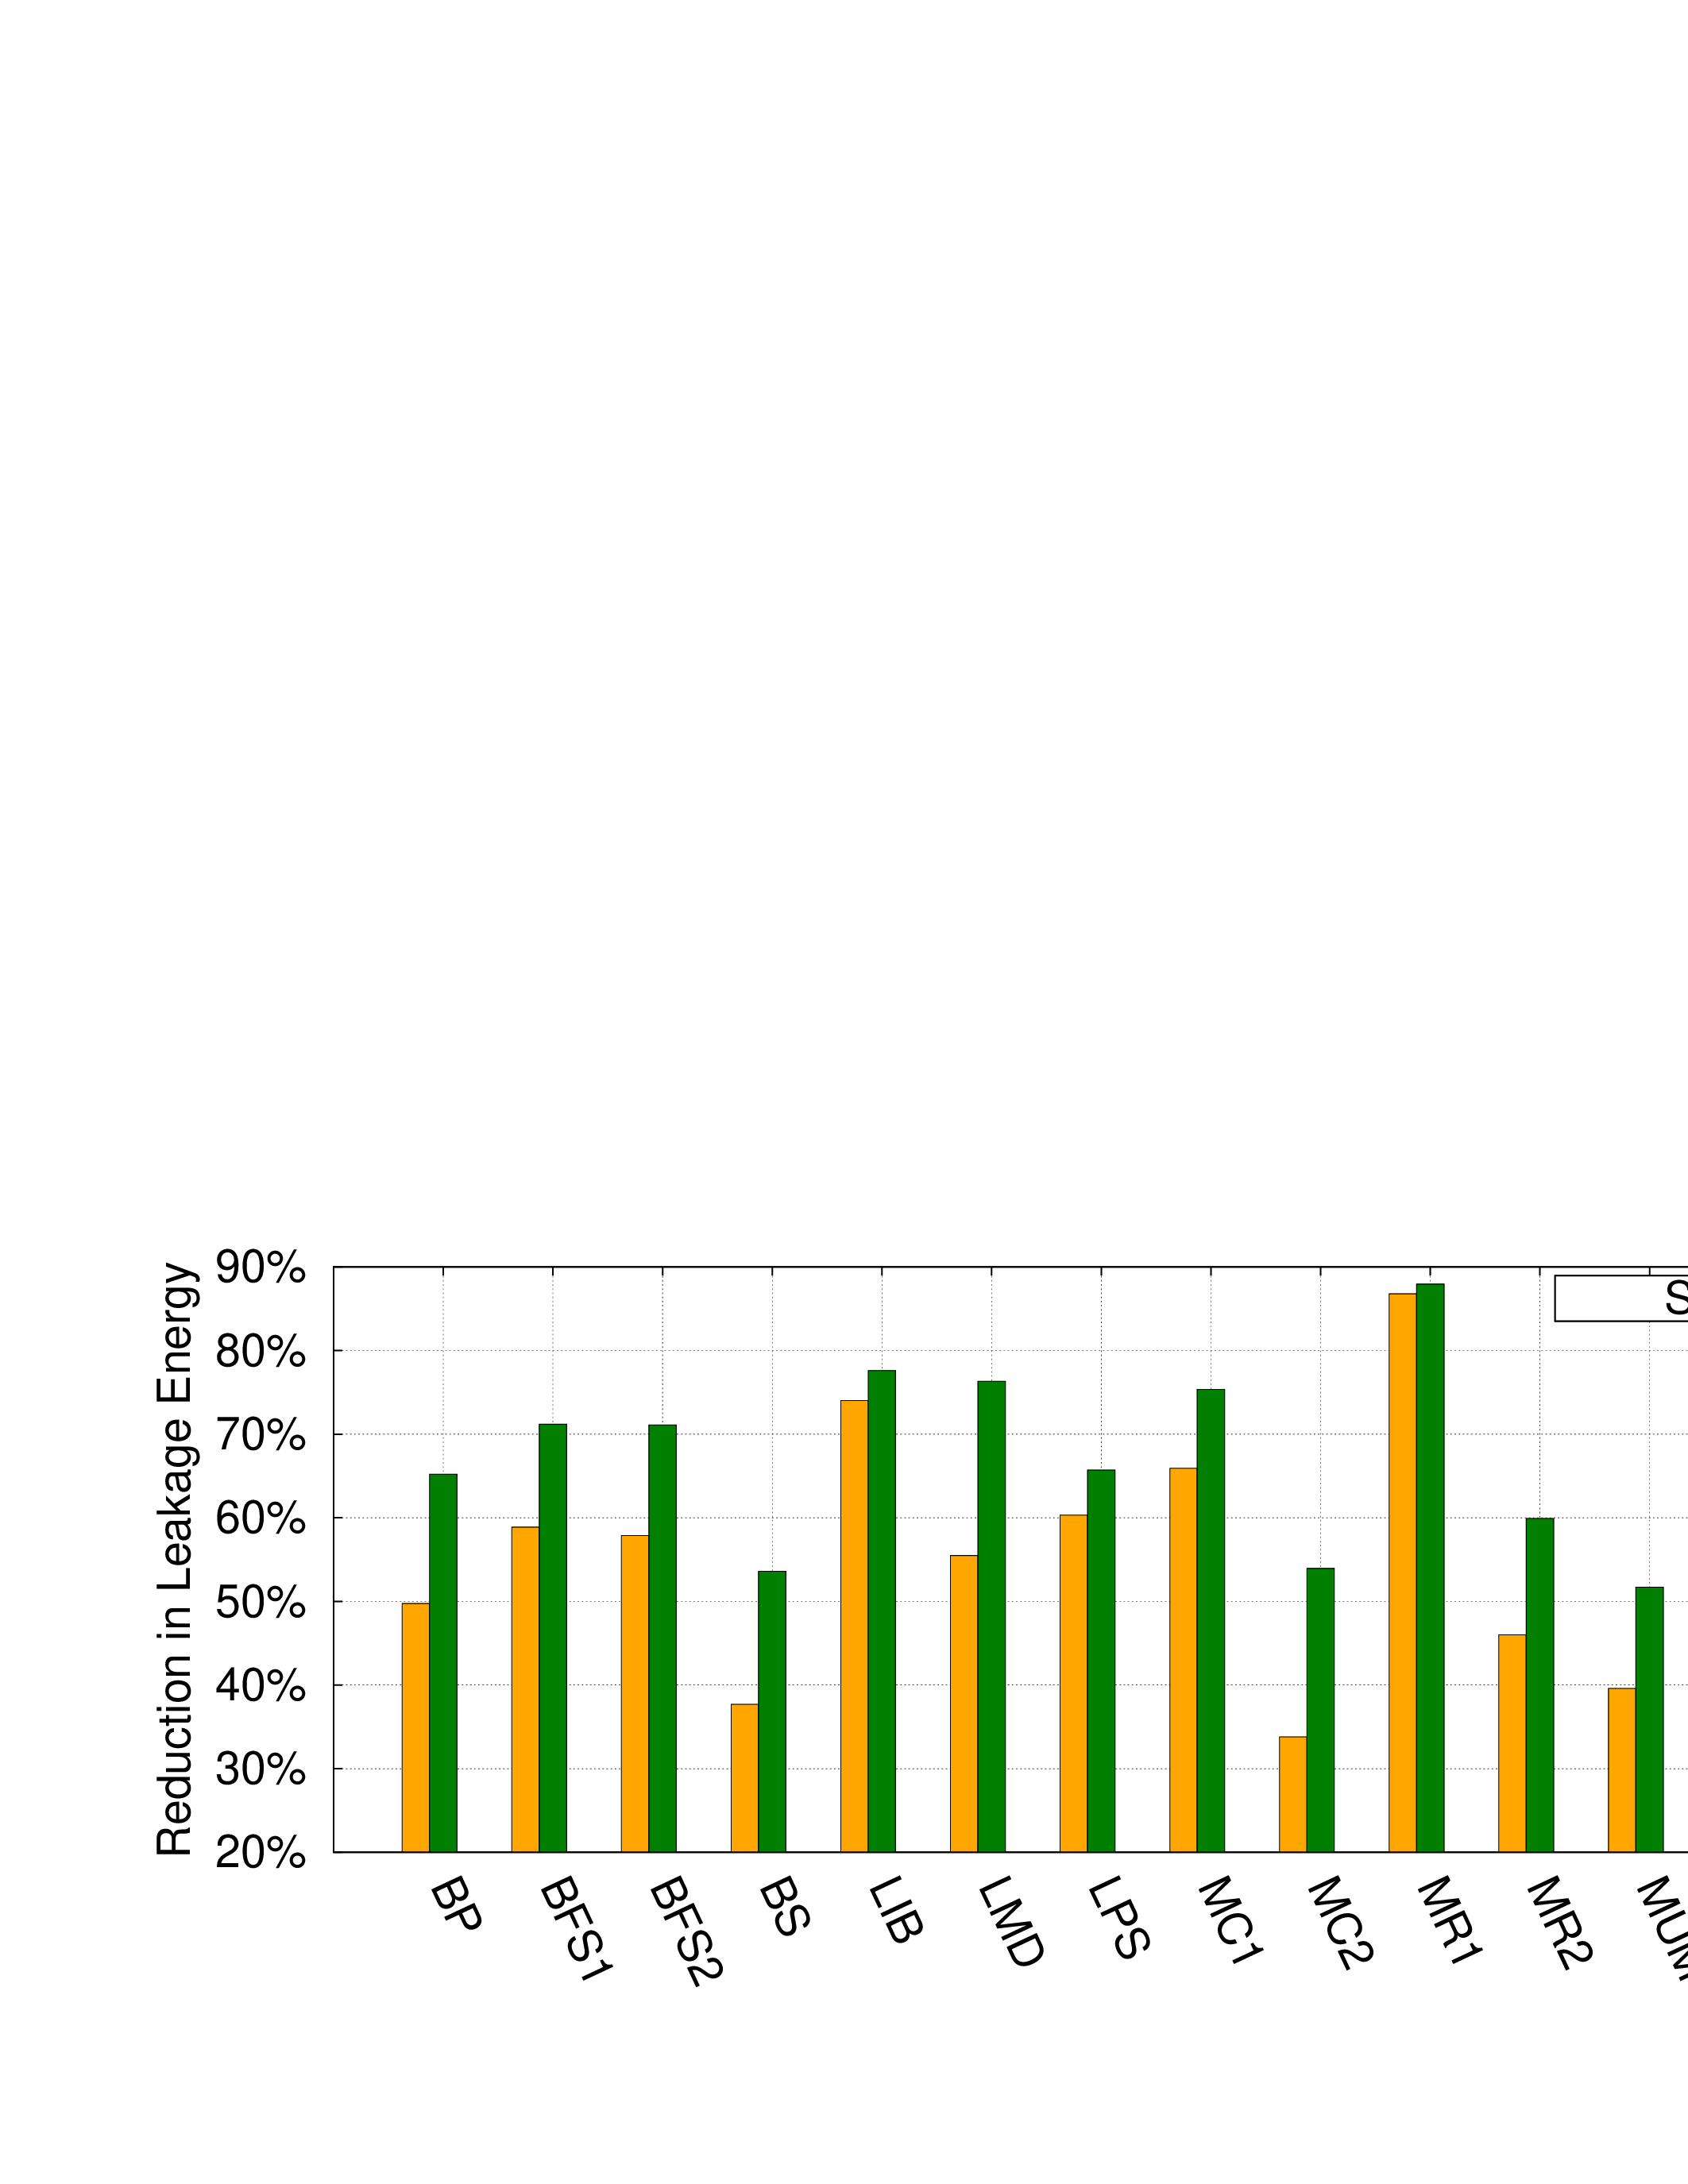}
\vskip -3mm
\caption{Comparing Leakage Energy with two-level Scheduler}
\label{fig:2Level}
\vskip -3mm
\end{figure*}

\section{Comparison with Different Schedulers}

Figure~\ref{fig:GTO} and \ref{fig:2Level} show the effectiveness of \emph{Power-OPT} when it is evaluated with GTO and two-level scheduling policies respectively. The figures  compare \emph{Power-OPT} and \emph{Sleep-Reg} with \emph{Baseline} by measuring the reduction in leakage energy for the corresponding scheduling policies. The results show that \emph{Power-OPT-GTO} and \emph{Power-OPT-two-level} achieve an average reduction leakage energy by 69.3\% and 69.65\% with respect to \emph{Baseline-GTO} and \emph{Baseline-two-level} respectively. With different scheduling policies, the warps in the SM have different interleaving patterns, which affect the distance between the two consecutive accesses to a register. Even with the change in these access patterns, \emph{Power-OPT} shows reduction in leakage energy when compared to \emph{Baseline} and \emph{Sleep-Reg}.  We also find that \emph{Baseline-GTO} performs better than \emph{Baseline-two-level} in terms of simulation cycles, hence \emph{Baseline-GTO} relatively consumes less leakage energy when compared to \emph{Baseline-two-level}. However, the average energy savings of \emph{Power-OPT} are not affected significantly even with change in the scheduler.

\begin{figure*}
        \begin{subfigure}[b]{1.0\textwidth}
        		\centering
                \includegraphics[scale=0.45]{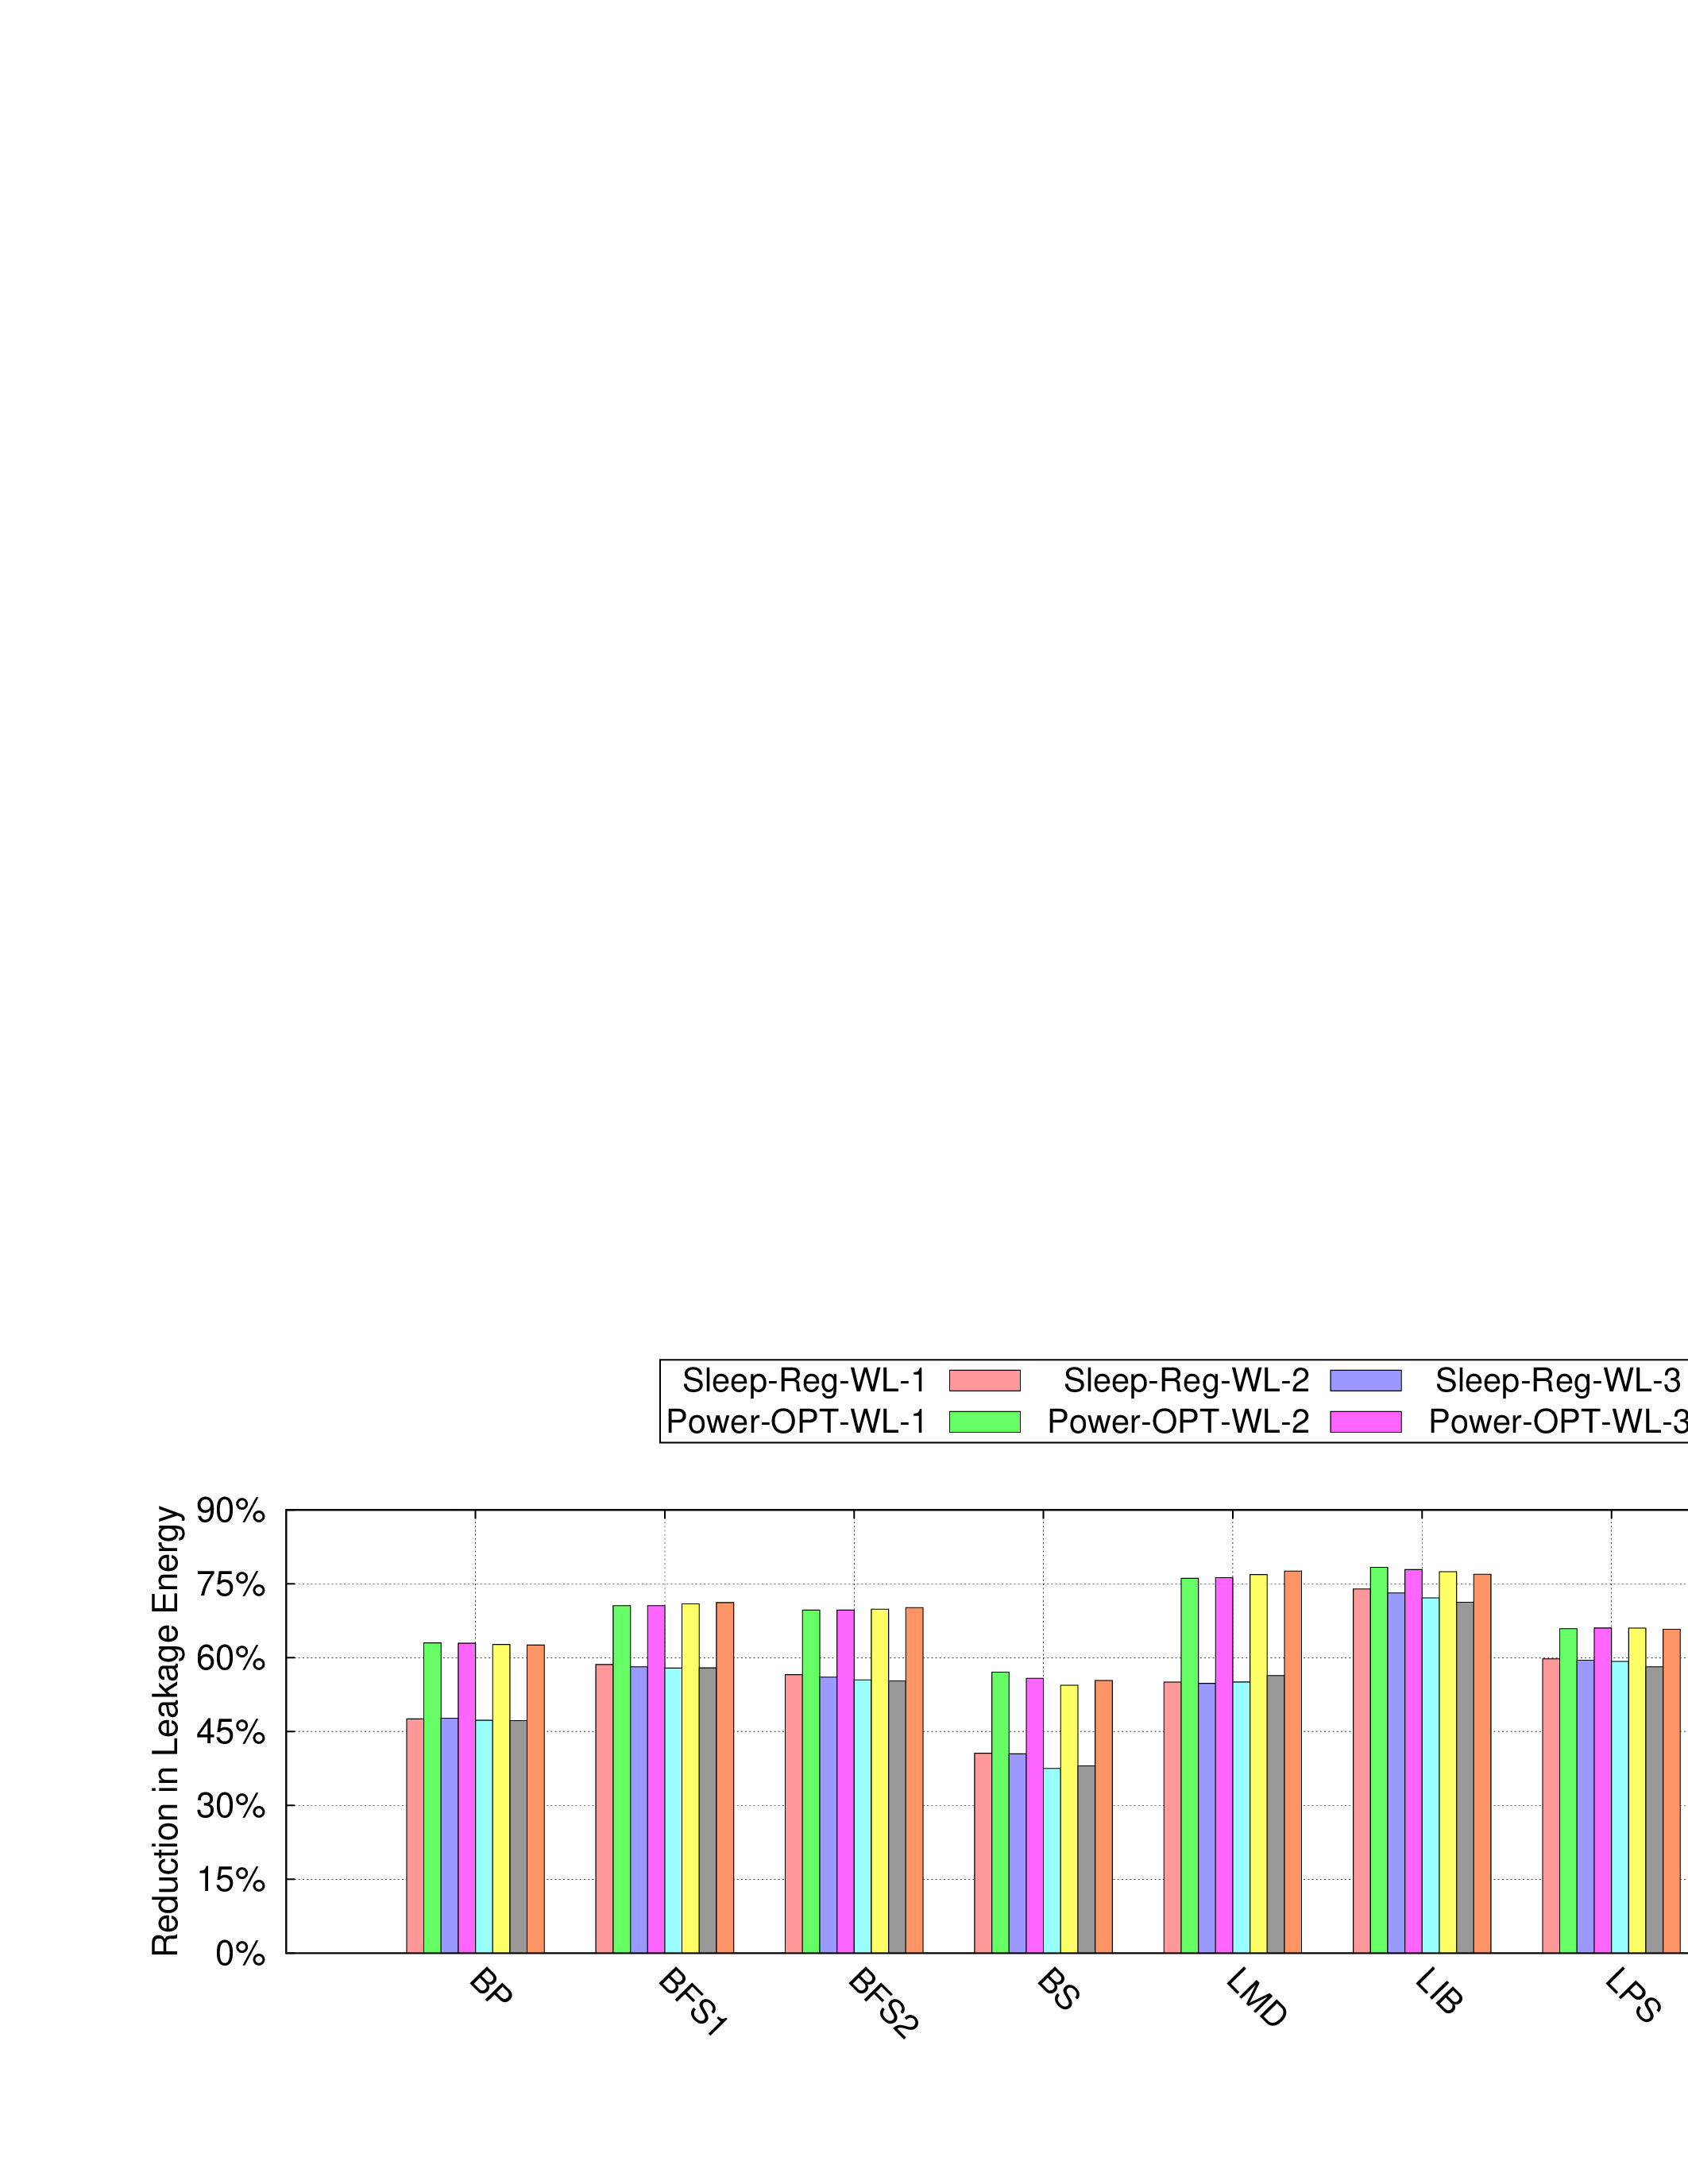}
                \caption{Part-1}
                \label{fig:wl_ener1}
        \end{subfigure}%
        \\
        \begin{subfigure}[b]{1.0\textwidth}
        \centering
                \includegraphics[scale=0.45]{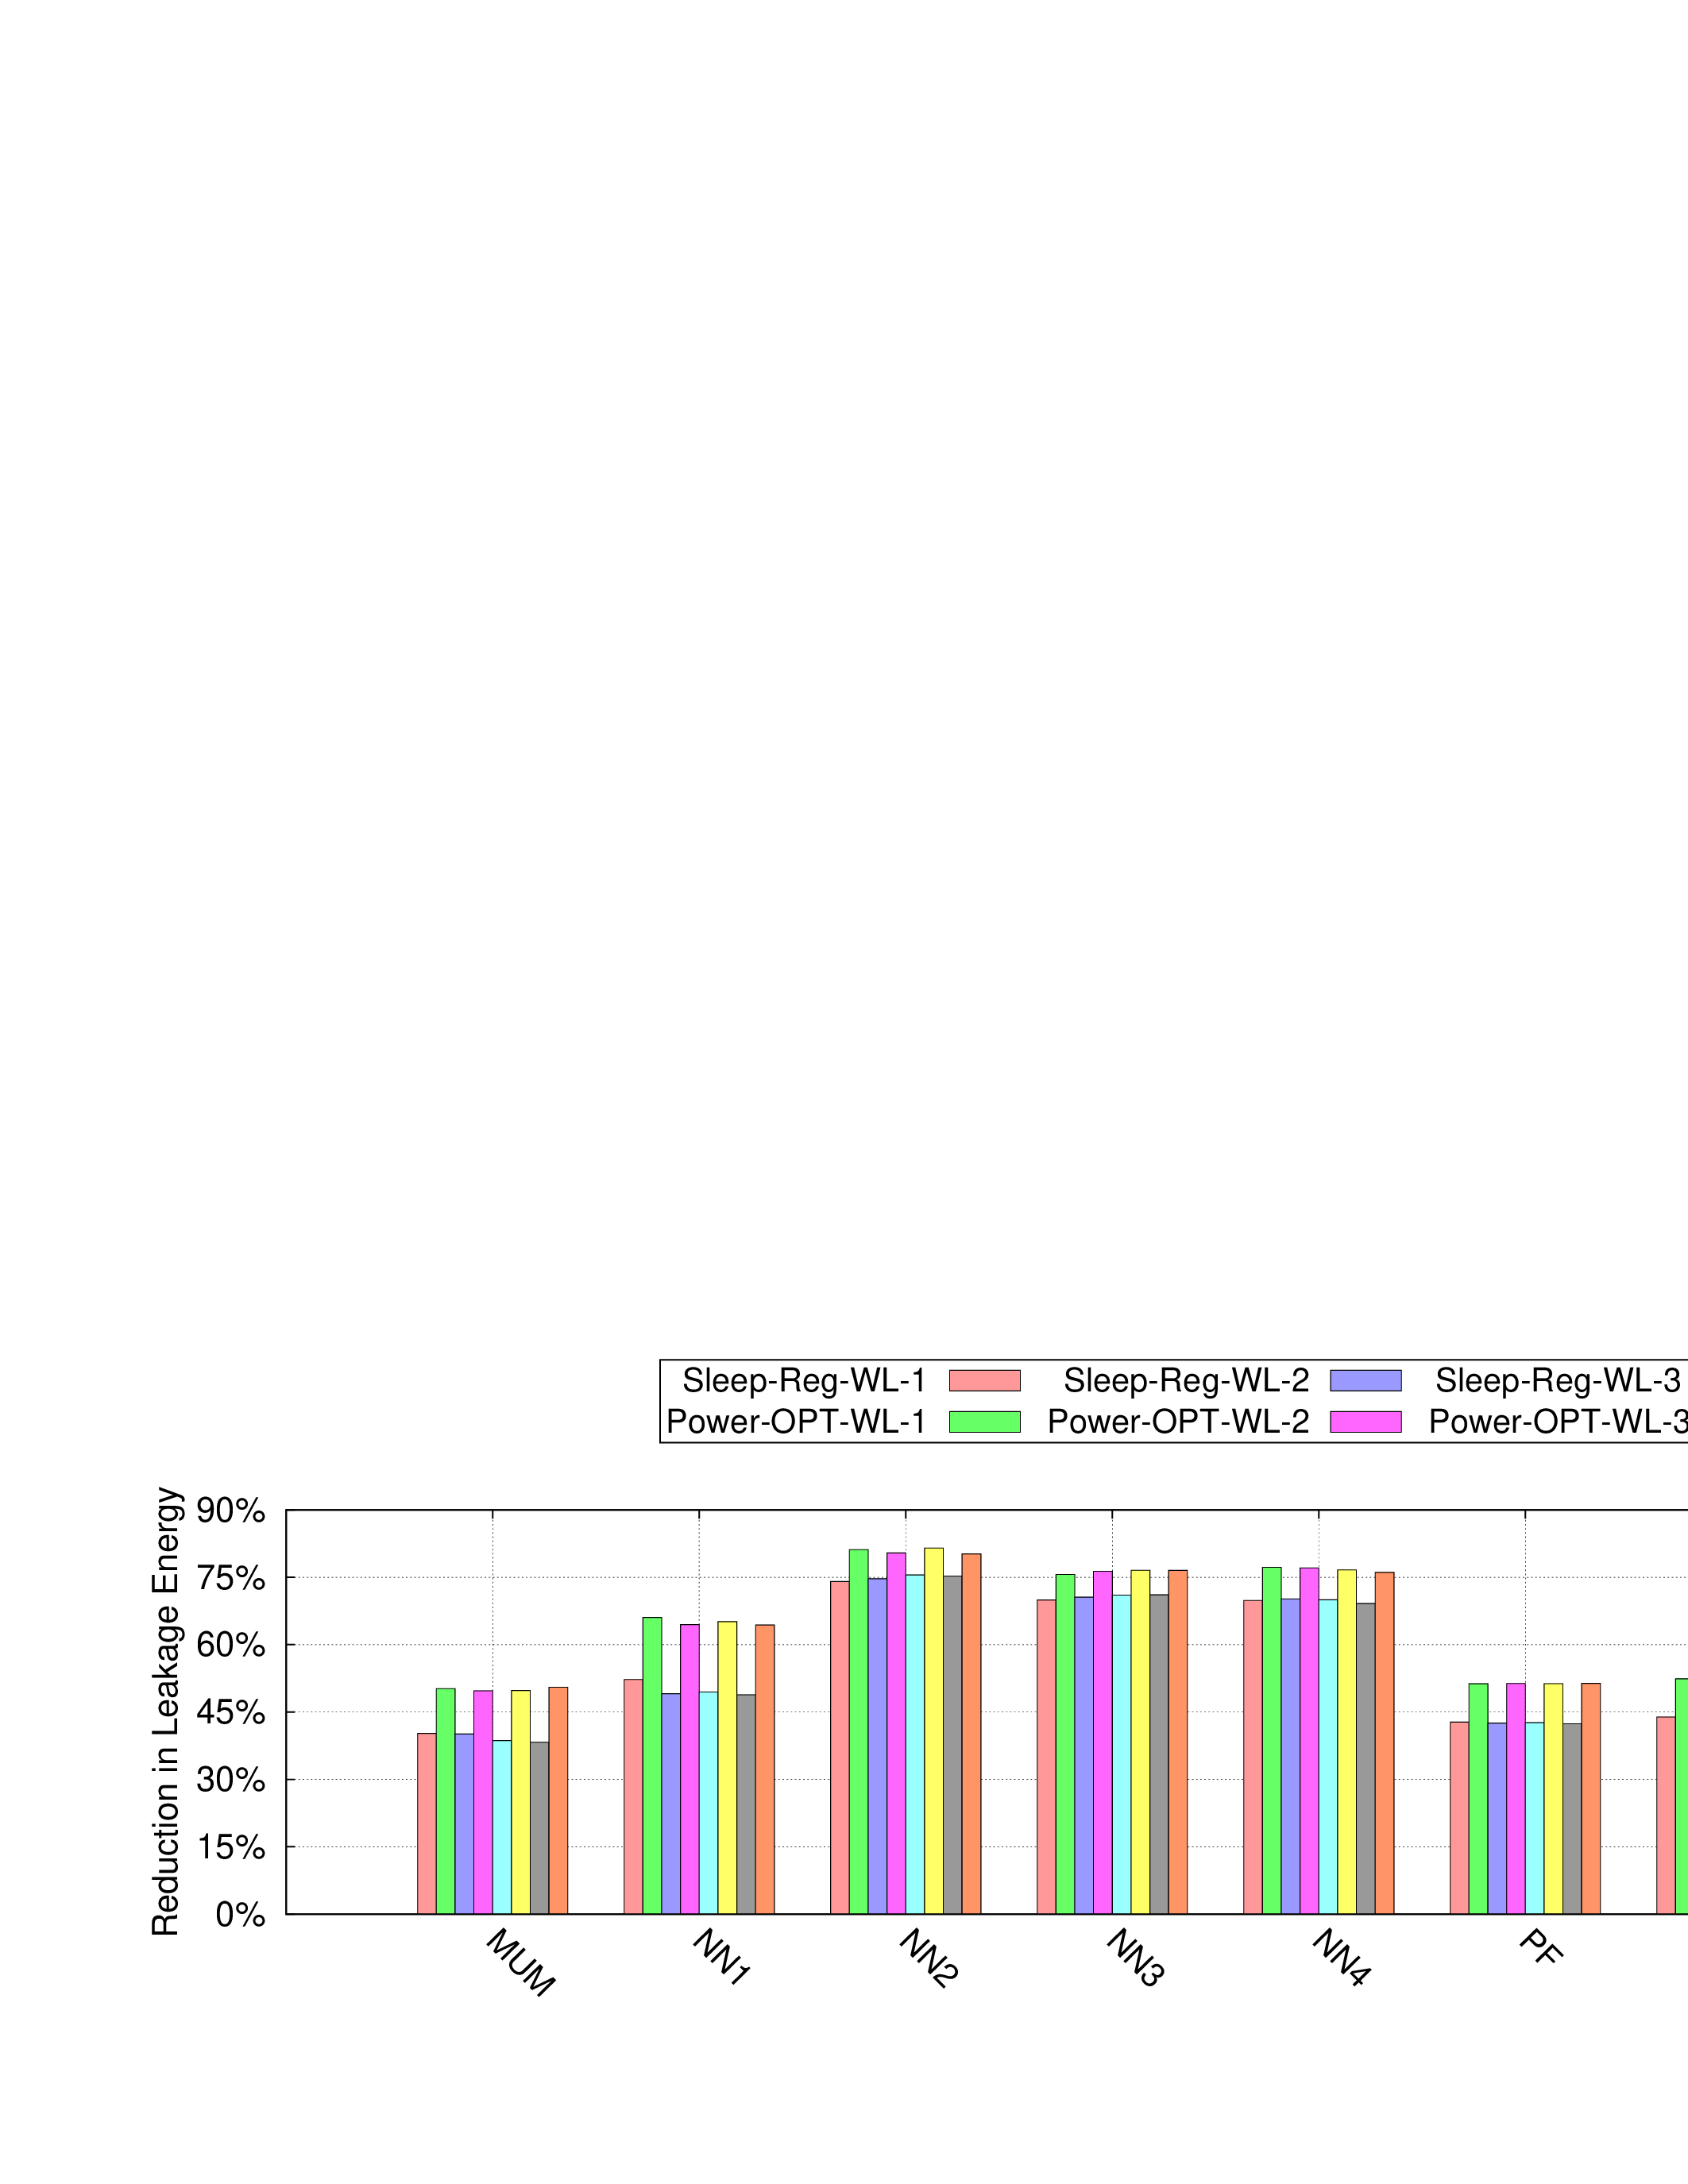}
                \caption{Part-2}
                \label{fig:wl_ener2}
        \end{subfigure}%
\vskip -3mm
\caption{Comparing the Leakage Energy for Various Wake Up Latencies}   
\label{fig:WakeupLatencies_energy}     
\vskip -3mm
\end{figure*}

\section{Comparing Leakage Energy for Various Threshold Distances } \label{sec:appendix}
\begin{table*}[t]
\caption{Comparing Register Leakage Energy by Varying Threshold Distance}
\vskip -3mm
\centering
\scalebox{0.7}{
\begin{tabular}{crrrrrrrrrrr}
  \hline\hline
Benchmark/ &1 &3 &5 &7 &9 &11 &13 &15 &17 &19 &21 \\ 
Threshold & & & & & & & & & & & \\ 
  \hline
BP & 161.35 & 157.53 & 160.15 & 159.24 & 160.37 & 159.31 & 159.77 & 158.76 & 158.76 & 158.17 & 158.17 \\ 
BFS1 & 24.35 & 24.41 & 24.37 & 24.37 & 24.37 & 24.37 & 24.37 & 24.37 & 24.37 & 24.37 & 24.37 \\ 
BFS2 & 9.48 & 9.48 & 9.48 & 9.48 & 9.48 & 9.48 & 9.48 & 9.48 & 9.48 & 9.48 & 9.48 \\ 
BS & 1,294.03 & 1,248.48 & 1,297.95 & 1,217.05 & 1,234.91 & 1,272.51 & 1,274.84 & 1,226.73 & 1,226.73 & 1,226.73 & 1,318.11 \\ 
LMD & 1.29 & 1.19 & 1.19 & 1.19 & 1.19 & 1.19 & 1.19 & 1.19 & 1.19 & 1.19 & 1.19 \\ 
LIB & 1,450.33 & 1,417.11 & 1,405.82 & 1,398.28 & 1,393.74 & 1,392.54 & 1,384.47 & 1,387.17 & 1,388.15 & 1,392.62 & 1,396.44 \\ 
LPS & 127.78 & 126.42 & 123.90 & 123.74 & 123.06 & 124.57 & 124.57 & 124.58 & 124.59 & 122.89 & 122.90 \\ 
MC1 & 13.97 & 13.11 & 13.92 & 13.11 & 13.46 & 13.36 & 13.36 & 13.36 & 13.36 & 13.36 & 13.36 \\ 
MC2 & 2,519.92 & 2,509.54 & 2,513.09 & 2,514.36 & 2,510.54 & 2,507.01 & 2,509.69 & 2,509.70 & 2,509.70 & 2,509.70 & 2,509.70 \\ 
MR1 & 0.45 & 0.45 & 0.45 & 0.45 & 0.45 & 0.45 & 0.45 & 0.45 & 0.45 & 0.45 & 0.45 \\ 
MR2 & 1,610.22 & 1,604.20 & 1,588.87 & 1,690.66 & 1,690.66 & 1,690.66 & 1,609.18 & 1,573.74 & 1,573.74 & 1,666.44 & 1,638.38 \\ 
MUM & 207.28 & 205.54 & 205.18 & 208.21 & 206.68 & 205.71 & 205.31 & 204.16 & 204.16 & 206.54 & 205.67 \\ 
NN1 & 35.86 & 33.27 & 33.90 & 33.67 & 33.55 & 34.53 & 33.52 & 33.52 & 34.61 & 34.61 & 34.61 \\ 
NN2 & 91.32 & 86.19 & 86.86 & 80.37 & 82.30 & 84.90 & 83.48 & 82.24 & 83.68 & 83.68 & 83.68 \\ 
NN3 & 1,181.92 & 1,095.75 & 1,096.35 & 1,097.49 & 1,046.82 & 1,003.42 & 1,003.22 & 1,003.88 & 1,001.88 & 1,001.88 & 1,001.88 \\ 
NN4 & 11.09 & 10.47 & 10.47 & 10.50 & 10.06 & 9.72 & 9.59 & 9.87 & 9.60 & 9.60 & 9.60 \\ 
PF & 175.20 & 173.19 & 173.42 & 173.12 & 173.29 & 173.33 & 173.84 & 174.83 & 174.83 & 174.04 & 174.04 \\ 
SP & 184.20 & 164.98 & 174.55 & 165.88 & 183.55 & 183.42 & 172.22 & 172.22 & 172.22 & 172.22 & 172.22 \\ 
SGEMM & 4,129.08 & 4,110.52 & 4,108.37 & 4,101.65 & 4,123.14 & 4,109.10 & 4,102.83 & 4,109.63 & 4,155.39 & 4,145.52 & 4,145.52 \\ 
SPMV & 21.86 & 21.67 & 21.57 & 21.61 & 21.67 & 21.90 & 21.89 & 22.27 & 22.31 & 22.30 & 22.30 \\ 
VA & 4.09 & 4.07 & 4.05 & 4.05 & 4.05 & 4.05 & 4.05 & 4.05 & 4.05 & 4.05 & 4.05 \\ \hline
\end{tabular}}
\label{table:threshold}
\end{table*}  

Table~\ref{table:threshold} shows the effect of threshold distance on register leakage energy for \emph{Power-OPT} approach. The results are collected by varying the threshold distance from 1 to 21. The table shows that keeping the threshold distance to 1 does not benefit with respect to energy consumption because with the shorter threshold distance, the registers of an instruction are turned to SLEEP or OFF state very soon, which leads to increase in the simulation cycles when there are frequent wakeup calls to the registers. Whereas, having a high threshold distance (i.e., distance 21) also does not help in minimizing energy because with longer distance, a register can be turned into SLEEP or OFF only when it is accessed after longer distance, this will result in losing the opportunity to save leakage energy. Hence, having the threshold distance at intermediate level can achieve more energy savings.

Consider the application \emph{SGEMM}, it achieves lowest energy at a threshold distance of 7. Further, with an increasing in the distance from 1 to 7, the leakage energy tends to decrease, and with an increasing in the distance beyond 7 tends to increase the energy. The similar behavior can be observed with \emph{BS, NN2, MC1, PF,} and \emph{SPMV} applications as well. However, some applications like \emph{BP, LIB, MC2,} and  \emph{MR2} achieve their minimum energy at a threshold distance other than 7.  For some applications like \emph{BFS1}, the leakage energy does not change beyond particular threshold distance because a register can be turned  into SLEEP or OFF state only up to a certain threshold distance, beyond that the register must be kept in the ON the state even with increasing the threshold distance.

Finally, we chose the threshold distance of 7 for the experiments in the paper, which achieves lowest energy for maximum number of applications. However, this value can be reconfigured depending on the application behavior.
